# Supplementary material for: AdBooster: Personalized Ad Creative Generation using Stable Diffusion Outpainting
Source: arXiv:2309.11507 source file (2023-09-08)
Supplement: Supplementary file 1 [file appendix.tex]

% where:
% \begin{itemize}
%     \item $\pi_{\theta + \epsilon}(\mathbf{a}|\mathbf{s})$ is the deterministic policy resulting from applying $epsilon$ noise to the original $\theta$ parameters of the score function: $\pi_{\theta + \epsilon}(\mathbf{a}|\mathbf{s}) = rank_{ \theta+ \epsilon}  (\mathbf{a}|\mathbf{s})$
% \end{itemize}

% \begin{equation}
% \begin{split}
%     \nabla_\theta \E_{\epsilon \sim N(0,I)} J(\theta + \sigma \epsilon)\} = \frac{1}{\sigma}\E \{ J(\theta + \sigma \epsilon)\epsilon \} 
% \end{split}
% \end{equation}

% \begin{equation}
%     \nabla_\theta J_{ES}(\theta) = \E_{\epsilon} \{ R(\mathbf{a}(\theta +  \epsilon),\mathbf{s})\nabla_\theta \log \pi_{\theta + \epsilon}(\mathbf{a}|\mathbf{s}) \}
% \end{equation}
% where:
% \begin{itemize}
%     \item $\pi_{\theta + \epsilon}(\mathbf{a}|\mathbf{s})$ is the deterministic policy resulting from applying $epsilon$ noise to the original $\theta$ parameters of the score function: $\pi_{\theta + \epsilon}(\mathbf{a}|\mathbf{s}) = rank_{ \theta+ \epsilon}  (\mathbf{a}|\mathbf{s})$
% \end{itemize}

% With a change of notation we have:


% \begin{equation}
%     \nabla_\theta J_{PG}(\theta) = \E_{\epsilon} \{ R(\mathbf{a}(\epsilon, \theta),\mathbf{s})\nabla_\theta \log \pi_{\theta,\epsilon}(\mathbf{a}|\mathbf{s}) \}
% \end{equation}
% where:
% \begin{itemize}
%     \item $\pi_{\theta,\epsilon}(\mathbf{a}|\mathbf{s})$ is the stochastic policy resulting from applying the softmax transform on the deterministic score function: $\pi_{\theta,\epsilon}(\mathbf{a}|\mathbf{s}) = \exp_{\epsilon} \{util_\theta (\mathbf{a},\mathbf{s})\}$  (here, $\epsilon$ is the seed for the random choice)
% \end{itemize}
